# Supplementary material for: MolScribe: Robust Molecular Structure Recognition with Image-To-Graph Generation
Source: arXiv:2205.14311 source file (2023-03-20)
Supplement: Supplementary file 1 [file appendix.tex]

\section{Experiment Details}
% Our code and data are available at \url{https://anonymous.4open.science/r/mol_img_rec/}.

\subsection{Computational Resource}
Our experiments are conducted on a Linux server with 96 CPUs and 500GB RAM. We use eight NVIDIA A100 GPUs to train our models. It takes 15 hours to train the model. Our neural network implementation is based on PyTorch~\cite{pytorch}. 

Our code can be found at \url{https://github.com/thomas0809/MolScribe}.
Our web interface (\url{https://huggingface.co/spaces/yujieq/MolScribe}) is implemented in Hugging Face as a Gradio space.\cite{gradio}

\subsection{Data}

\paragraph{Train}
The synthetic training data is constructed with molecules sampled from PubChem (\url{https://ftp.ncbi.nlm.nih.gov/pubchem/Compound/}) and images automatically rendered by Indigo. Unlike previous work, we do not apply any filtering based on molecule size or other properties, but randomly sample the molecules. We make a few changes to the source code of Indigo to support more rendering options and obtain pixel-level atom coordinates. The changed codes are included in our codebase.

The patent training data is downloaded from USPTO, Grant Red Book section (\url{https://bulkdata.uspto.gov/}). We collect the MOLfiles and corresponding images, and use RDKit to convert molecules into SMILES strings. Relative coordinates, bond types, and superatom labels (functional group abbreviations, R-groups) are parsed from the MOLfiles.

\paragraph{Test}
The synthetic image benchmarks are automatically generated by two chemistry toolkits, Indigo and ChemDraw. We use the same set of molecules from the USPTO benchmark\cite{rajan2020review} to generate the images.
% In the synthetic experiment, we construct four test sets with different molecule distributions and image distributions. We sample molecules from PubChem (P) and USPTO (U), and generate images with Indigo (I) and ChemDraw (C). 

The realistic image benchmarks are taken from \citeauthor{rajan2020review} and \citeauthor{mse-staker}. CLEF, UOB, and USPTO are downloaded from \url{https://github.com/Kohulan/OCSR_Review}, and Staker is downloaded from \url{https://drive.google.com/drive/folders/16OjPwQ7bQ486VhdX4DWpfYzRsTGgJkSu}. The perturbed datasets are constructed by \citeauthor{img2mol}, available at \url{https://github.com/bayer-science-for-a-better-life/Img2Mol/}. 
We further create a new benchmark ACS with molecular images from chemistry literature. We randomly sample molecular images cropped from chemistry publications, and ask chemists to manually label their SMILES.

\Cref{fig:bench} shows the example images in our benchmarks. The processed datasets can be downloaded at \url{https://github.com/thomas0809/MolScribe#data}.
 
% The molecular images used in the human evaluation are sampled from the Valko dataset~\cite{staker2019molecular}.

\begin{figure}[t]
    \centering
    \includegraphics[width= \linewidth]{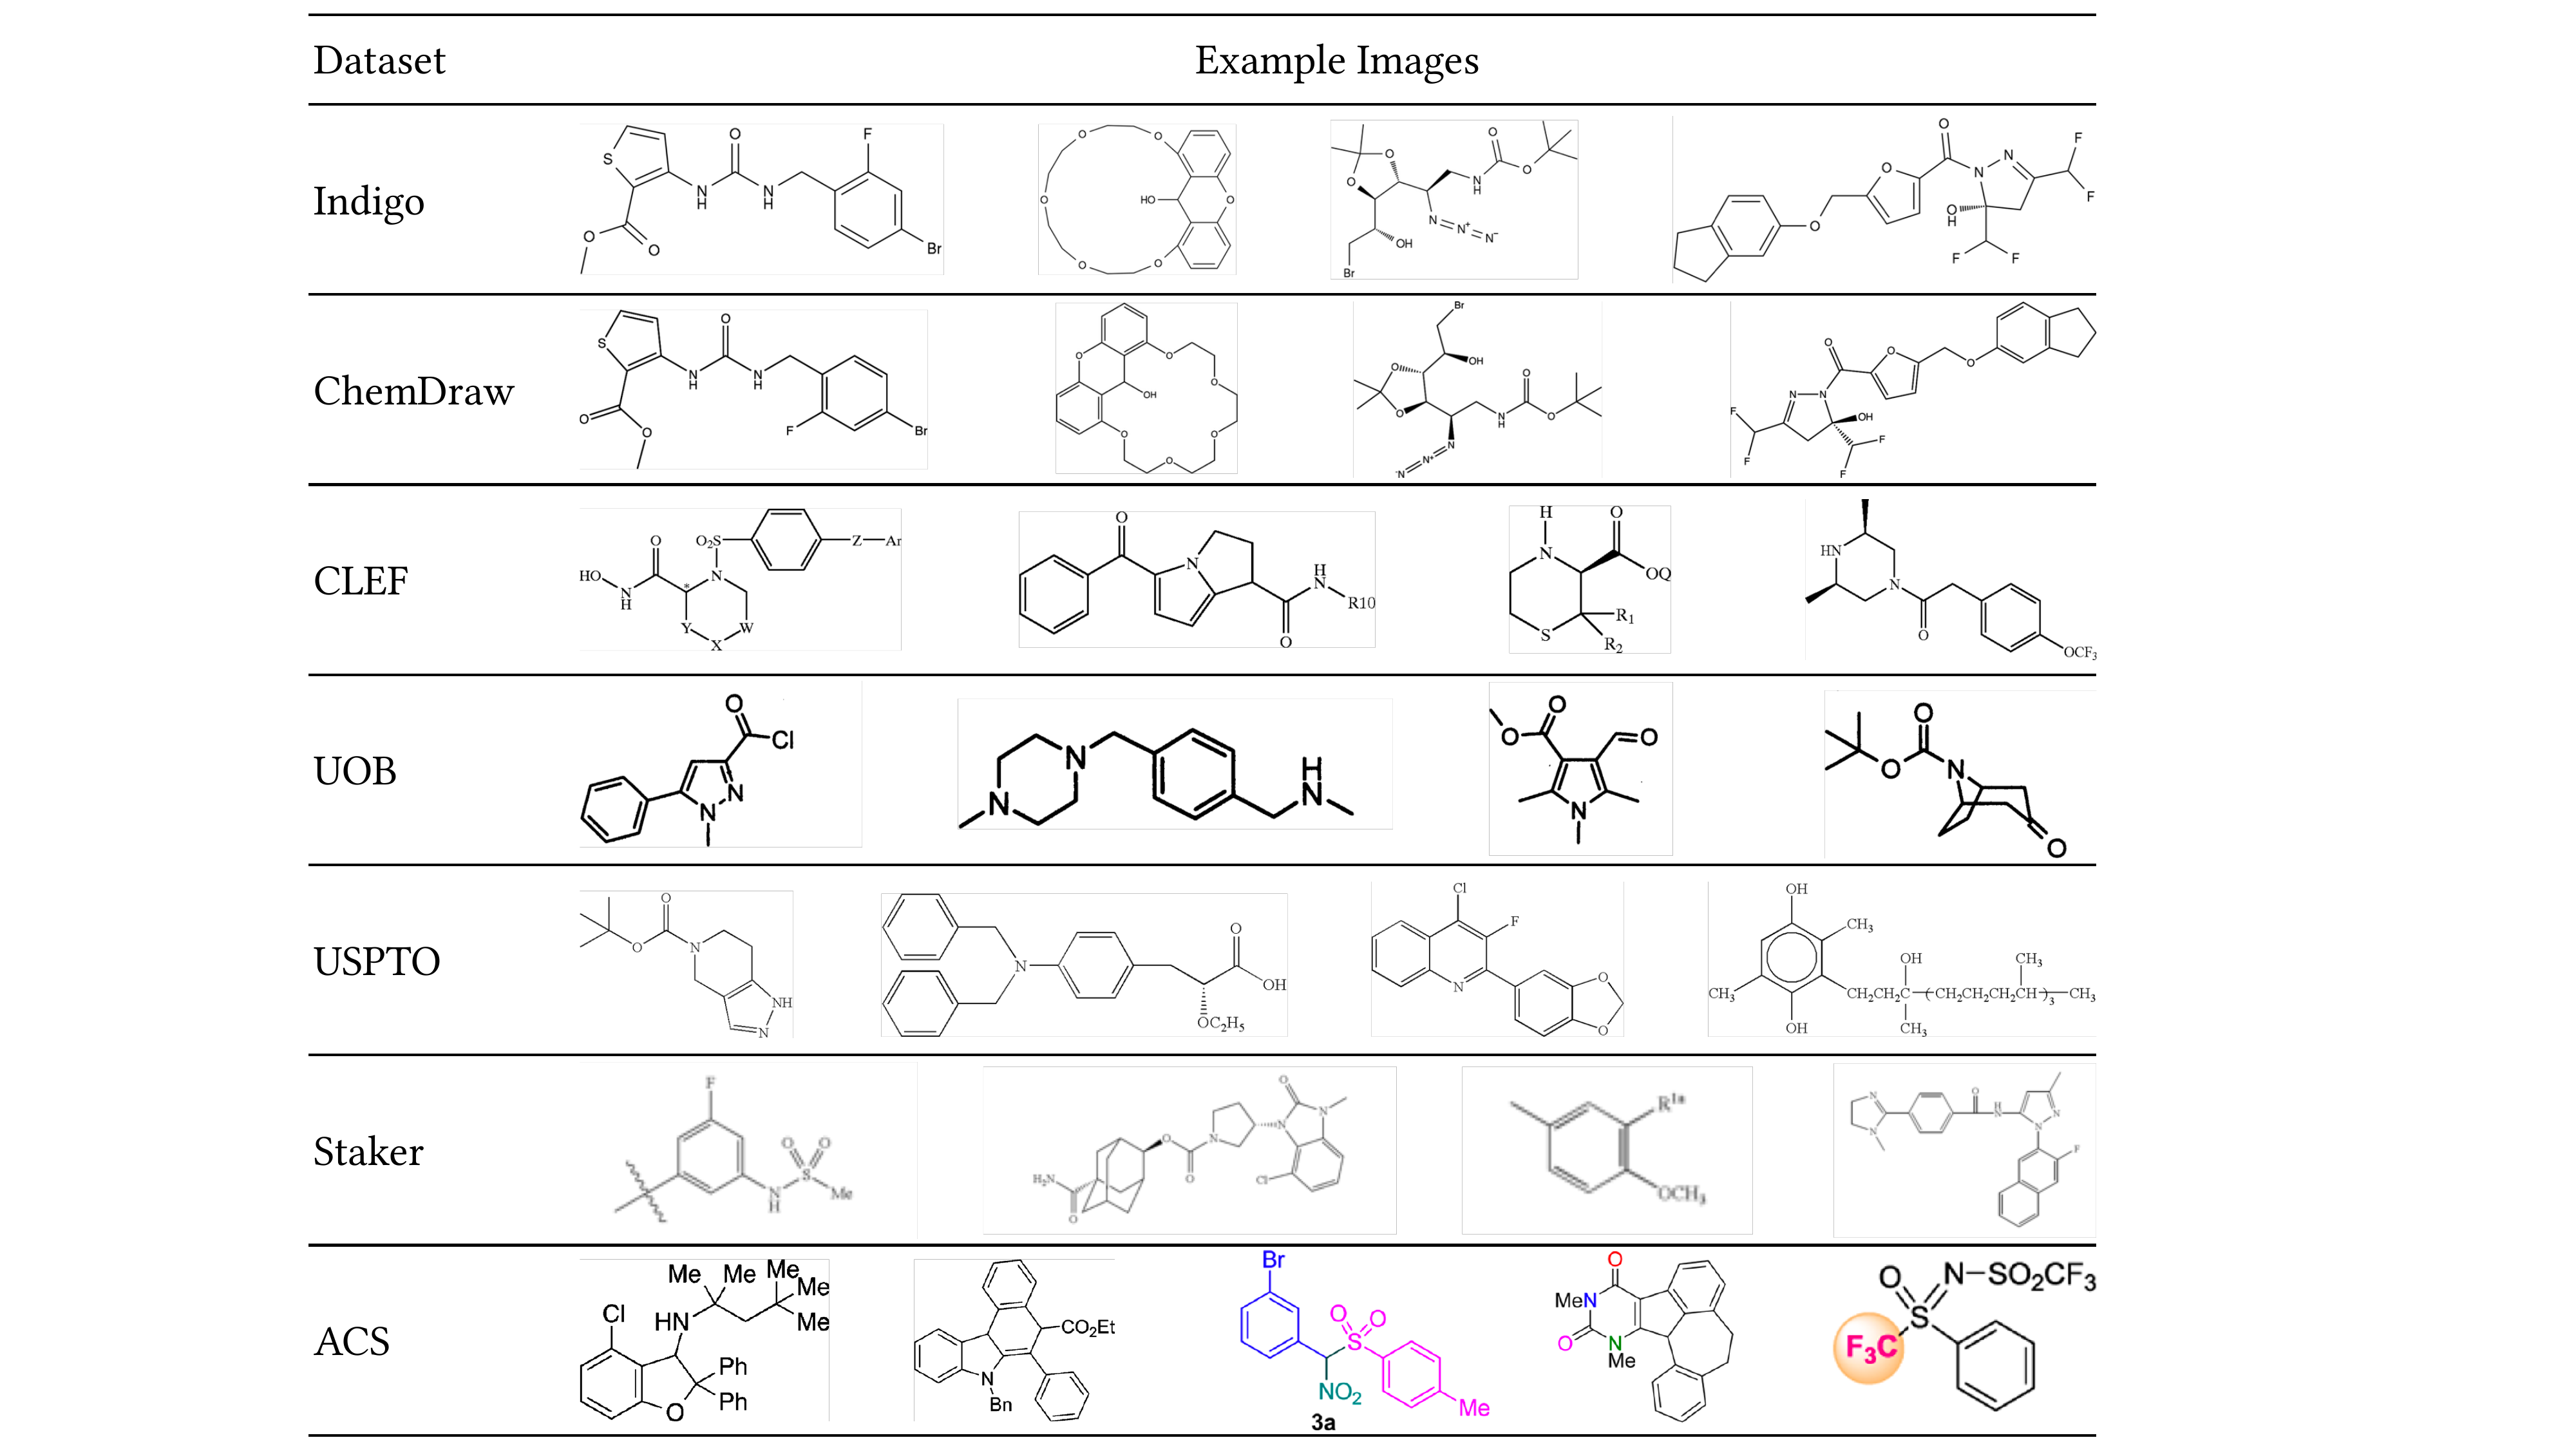}
    \vspace{-0.1in}
    \caption{Example molecular images in the test sets. The first two rows are synthetic images rendered by Indigo and ChemDraw. CLEF, UOB, USPTO, Staker, and ACS are datasets with realistic images.}
    \label{fig:bench}
\end{figure}

\subsection{Data Augmentation}
\paragraph{Molecule Augmentation}
Indigo can automatically render images of molecules, but never uses abbreviations or R-groups. In order for the synthetic images to cover more molecular patterns, we design molecule augmentation strategies:
\begin{itemize}
    \item Abbreviation: We compile a list of 53 common functional group substitution rules, and randomly replace functional groups with their abbreviations in the training data. It is implemented by the substructure matching function in Indigo. The full substitution list can be found in our codebase.
    \item R-group: We randomly add R-group atoms to the training molecules. The R-group label is randomly sampled from the list $[R, R_1, R_2, \dots, R_{12}, R_a, R_b, R_c, \allowbreak R_d, X, Y, Z,\allowbreak A, Ar]$.
    \item Aromaticity: We randomly draw aromatic rings in circles or lines.
    \item Explicit Hydrogens: We randomly add hydrogen as explicit atoms.
\end{itemize}
% Functional groups are often presented as abbreviated labels in molecular images. %\Cref{tab:functional} shows a few common abbreviations.
% However, 
% If such patterns are never seen during training, we cannot expect the model to understand their corresponding substructure. 

\paragraph{Image Augmentation}
The synthetic images are dynamically rendered by Indigo during training, with the following options:
\begin{itemize}
    \item render-background-color: 1,1,1;
    \item render-relative-thickness: randomly sampled from $[0.8, 2]$;
    \item render-bond-line-width: randomly sampled from $[1,3]$;
    \item render-font-family: randomly chosen from \{Arial, Times, Courier, Helvetica\};
    \item render-label-mode: randomly chosen from \{hetero, terminal-hetero\};
    \item render-implicit-hydrogens-visible: randomly chosen from \{true, false\}. 
\end{itemize}

We also apply image augmentation during training, including the following operations to the image:
\begin{itemize}
    \item rotate by a random angle from $[-90^{\circ}, 90^{\circ}]$;
    \item crop each side of the image by at most 1\%;
    \item pad one side of the image by at most 40\%;
    \item downscale the image by 20--50\% and upscale back;
    \item blur the image using a random-sized kernel;
    \item add Gaussian noise to the image;
    \item add salt-and-pepper noise (random black pixels) to the image.
\end{itemize}
The image augmentations are implemented based on Albumentations~\cite{buslaev2020albumentations}. 

The rendering options and augmentation operations are chosen such that the augmented images have different styles and qualities, and preserve the necessary information for human to understand the molecule structure. %\Cref{fig:aug} shows some examples.

\subsection{Expansion of Abbreviated Structures}

The algorithm presented in Algorithm \ref{algo:condensed} of the main manuscript makes three assumptions: 1) the structure of the functional group consists of a single-chain backbone to which side atoms are attached; 2) the atoms in the formula are listed in order down the chain; and 3) every atom has a uniquely defined valence. (For example, for a backbone XY with side atoms A attached to X and B, C attached to Y, we assume the formula can be written written XAYBC or XAYCB.)  In the full algorithm, we further address the following cases:
\begin{enumerate}
    \item \textit{Carbon chains}. A chain of carbons with homogeneous side atoms is often written $\mathrm{C}_a\mathrm{X}_b$ instead of $\mathrm{C}\mathrm{X}_k \mathrm{C}\mathrm{X}_k\ldots$, where $\mathrm{X}$ is usually hydrogen or a halogen. This issue is handled by splitting any occurrence of $\mathrm{C}_a\mathrm{X}_b$ to $\mathrm{C}\mathrm{X}_q \ldots \mathrm{C}\mathrm{X}_q \mathrm{C}\mathrm{X}_{q+r}$ where $q$ and $r$ are the quotient and remainder upon dividing $b$ by $a$.

    \item \textit{Abbreviations}. The formulas often have abbreviations within them (e.g.\ Me, Et). They are treated as superatoms with an equivalent valence. In the end, they are expanded to recover their original graph structure.

    \item \textit{Nested formulas}. The formulas can be nested (e.g.\ $\mathrm{N}(\mathrm{CH}_3)_2$). Similar to abbreviations, we treat the nested formula as superatoms. We assume they are attached to the backbone with a single bond. We then recursively apply our algorithm to the nested formula to obtain its structure and attach it to the current atom. 
    If the superatom does not saturate the valence of the current atom, we additionally require that the superatom's implicit valence has become 0 as we will not attach anything else to it. If it's not 0, we return FAILURE.
    On the other hand, if the current atom's valence becomes saturated, the superatom becomes the new current atom.

    \item \textit{Multiple valences}. Some atoms have multiple possible valences. To handle this, we try each possible valence until we succeed. We try common valences before rare ones and higher valences before lower ones.
\end{enumerate}
